# Supplementary material for: Dynamics of an internally actuated weakly elastic sphere in a general quadratic flow
Source: arXiv:2512.08408 ancillary file (2025-12-09)
Supplement: Supplementary file 1 [file ESI_1.pdf]

## Dynamics of an internally actuated weakly elastic sphere in general quadratic flow

Shashikant Verma<sup>a</sup> and Navaneeth K. Marath<sup>\*ab</sup>

<sup>a</sup>Department of Mechanical Engineering, Indian Institute of Technology Ropar, 140001, India

<sup>b</sup>Centre of Research for Energy Efficiency and Decarbonization (CREED), Indian Institute of Technology Ropar, 140001, India; Email\*: navaneeth@iitrpr.ac.in

### 1 Particle translating in the general quadratic flow

The components of the disturbance velocity and the pressure fields in the fluid at leading-order are obtained as

$$v_{d_q,r}^{(0)} = \frac{1}{160\xi^5} \left[ 4 \cos \theta (5\gamma_{333}(-5 + 7\xi^2) + 4\xi^2(-5 - 5\xi^2(-3 + \tau) + 3\tau) + 25\gamma_{333}(5 - 7\xi^2) \cos 2\theta \right. \\ \left. + 30(-5 + 7\xi^2) \sin^2 \theta ((2\gamma_{223} + \gamma_{333}) \cos 2\phi - 2\gamma_{123} \sin 2\phi)) + 5(-5 + 7\xi^2)(4(4\gamma_{122} + \gamma_{133}) \right. \\ \left. \times \cos 3\phi \sin^3 \theta - 3\gamma_{133} \cos \phi (\sin \theta + 5 \sin 3\theta) - 3\gamma_{233}(\sin \theta + 5 \sin 3\theta) \sin \phi + 4(4\gamma_{222} \right. \\ \left. + 3\gamma_{233}) \sin^3 \theta \sin 3\phi) \right], \quad (1)$$

$$v_{d_q,\theta}^{(0)} = \frac{1}{1920\xi^5} \left[ 4 \sin \theta (45\gamma_{333}(15 - 7\xi^2) + 24\xi^2(-5 + 5\xi^2(-3 + \tau) + 3\tau) - 5(-45(2\gamma_{223} + \gamma_{333}) \right. \\ \left. + (-32Q_{12} + 21(2\gamma_{223} + \gamma_{333}))\xi^2) \cos 2\phi + 10(-45\gamma_{123} + (-8Q_{11} + 8Q_{22} + 21\gamma_{123})\xi^2) \sin 2\phi \right. \\ \left. - 15(-15 + 7\xi^2) \cos 2\theta (5\gamma_{333} + 3(2\gamma_{223} + \gamma_{333}) \cos 2\phi - 6\gamma_{123} \sin 2\phi) + 10 \cos \theta ((64Q_{23}\xi^2 \right. \\ \left. + 21\gamma_{133}(15 - 7\xi^2) + 45\gamma_{133}(-15 + 7\xi^2) \cos 2\theta) \cos \phi - 6(4\gamma_{122} + \gamma_{133})(-15 + 7\xi^2) \cos 3\phi \right. \\ \left. \times \sin^2 \theta + (315\gamma_{233} - (64Q_{13} + 147\gamma_{233})\xi^2 + 45\gamma_{233}(-15 + 7\xi^2) \cos 2\theta) \sin \phi - 6(4\gamma_{222} \right. \\ \left. + 3\gamma_{233})(-15 + 7\xi^2) \sin^2 \theta \sin 3\phi) \right], \quad (2)$$

$$v_{d_q,\phi}^{(0)} = \frac{1}{192\xi^5} \left[ (9\gamma_{233}(-15 + 7\xi^2) + (-225\gamma_{233} + (-64Q_{13} + 105\gamma_{233})\xi^2) \cos 2\theta) \cos \phi - 6(4\gamma_{222} + 3\gamma_{233}) \right. \\ \left. \times (-15 + 7\xi^2) \cos 3\phi \sin^2 \theta - 48(Q_{11} + Q_{22})\xi^2 \sin 2\theta + 8(-45\gamma_{123} + (-2Q_{11} + 2Q_{22} + 21\gamma_{123}) \right. \\ \left. \times \xi^2) \cos 2\phi \sin 2\theta + (9\gamma_{133}(15 - 7\xi^2) + (225\gamma_{133} - (64Q_{23} + 105\gamma_{133})\xi^2) \cos 2\theta) \sin \phi + 4(-45 \right. \\ \left. \times (2\gamma_{223} + \gamma_{333}) + (-8Q_{12} + 42\gamma_{223} + 21\gamma_{333})\xi^2) \sin 2\theta \sin 2\phi + 6(4\gamma_{122} + \gamma_{133})(-15 + 7\xi^2) \right. \\ \left. \times \sin^2 \theta \sin 3\phi \right] \quad (3)$$

and

$$p_{d_q}^{(0)} = \frac{1}{64\xi^4} \left[ -105\gamma_{133} \cos \phi \sin \theta + 4 \cos \theta (35\gamma_{333} - 8\xi^2(-3 + \tau) - 175\gamma_{333} \cos 2\theta + 210(2\gamma_{223} + \gamma_{333}) \right. \\ \left. \times \cos 2\phi \sin^2 \theta) + 35(4(4\gamma_{122} + \gamma_{133}) \cos 3\phi \sin^3 \theta - 3(5 \sin 3\theta (\gamma_{133} \cos \phi + \gamma_{233} \sin \phi) + \sin \theta (\gamma_{233} \right. \\ \left. \times \sin \phi + 8\gamma_{123} \sin 2\theta \sin 2\phi)) + 4(4\gamma_{222} + 3\gamma_{233}) \sin^3 \theta \sin 3\phi) \right], \quad (4)$$

respectively. Here,  $\gamma_{ijk}$  and  $Q_{lm}$  with  $i, j, k = 1, 2, 3$  and  $l, m = 1, 2, 3$  are the Cartesian components of  $\gamma$  and  $\mathbf{Q}$ , respectively and  $\tau_l = \tau \hat{\mathbf{k}}$ . The components of the displacement at  $O(\alpha)$  are obtained as

$$u_{q,r}^{(1)} = \frac{1}{256\xi} \left[ \frac{1}{(2+\Gamma)(2+3\Gamma)} 4 \cos \theta (-3\Gamma^2(\xi^3(32+35\gamma_{333}-32\tau)+32(-3+\tau))-8\Gamma(-96+35\gamma_{333}\xi^3-8(-4+\xi^3)\tau)-4(32(-3+\tau)+\xi^3(-24+35\gamma_{333}+40\tau))+35(2+\Gamma)(2+3\Gamma)\xi^3(5\gamma_{333}\cos 2\theta-6(2\gamma_{223}+\gamma_{333})\cos 2\phi\sin^2\theta))+35\xi^3(-4(4\gamma_{122}+\gamma_{133})\cos 3\phi\sin^3\theta+3\gamma_{233}(\sin\theta+5\sin 3\theta)\times\sin\phi+3\cos\phi(\gamma_{133}\sin\theta+5\gamma_{133}\sin 3\theta+32\gamma_{123}\cos\theta\sin^2\theta\sin\phi)-4(4\gamma_{222}+3\gamma_{233})\sin^3\theta\times\sin 3\phi) \right] - \frac{P_0\xi}{2+3\Gamma}, \quad (5)$$

$$u_{q,\theta}^{(1)} = -\frac{1}{384\xi} \left[ \frac{2\sin\theta}{(2+\Gamma)(2+3\Gamma)} (864+1584\Gamma+432\Gamma^2-864\xi^3-1440\Gamma\xi^3-576\Gamma^2\xi^3+1260\gamma_{333}\xi^3+2520\Gamma\gamma_{333}\xi^3+945\Gamma^2\gamma_{333}\xi^3-288\tau-528\Gamma\tau-144\Gamma^2\tau+1440\xi^3\tau+1824\Gamma\xi^3\tau+576\Gamma^2\xi^3\tau+5(4+8\Gamma+3\Gamma^2)(64Q_{12}+42\gamma_{223}+21\gamma_{333})\xi^3\cos 2\phi-640Q_{11}\xi^3\sin 2\phi+640Q_{22}\xi^3\sin 2\phi-1280Q_{11}\Gamma\xi^3\sin 2\phi+1280Q_{22}\Gamma\xi^3\sin 2\phi-480Q_{11}\Gamma^2\xi^3\sin 2\phi+480Q_{22}\Gamma^2\xi^3\sin 2\phi-840\gamma_{123}\times\xi^3\sin 2\phi-1680\Gamma\gamma_{123}\xi^3\sin 2\phi-630\Gamma^2\gamma_{123}\xi^3\sin 2\phi+105(4+8\Gamma+3\Gamma^2)\xi^3\cos 2\theta(5\gamma_{333}+3(2\gamma_{223}+\gamma_{333})\cos 2\phi-6\gamma_{123}\sin 2\phi))+5\xi^3\cos\theta((128Q_{23}+147\gamma_{133}-315\gamma_{133}\cos 2\theta)\cos\phi+42(4\gamma_{122}+\gamma_{133})\cos 3\phi\sin^2\theta-128Q_{13}\sin\phi+147\gamma_{233}\sin\phi-315\gamma_{233}\cos 2\theta\sin\phi+168\gamma_{222}\times\sin^2\theta\sin 3\phi+126\gamma_{233}\sin^2\theta\sin 3\phi) \right], \quad (6)$$

and

$$u_{q,\phi}^{(1)} = \frac{5}{384}\xi^2 \left[ 63\gamma_{233}\cos\phi-63\gamma_{133}\sin\phi+\cos 2\theta((128Q_{13}+105\gamma_{233})\cos\phi+(128Q_{23}-105\gamma_{133})\sin\phi)+4\sin 2\theta(24(Q_{11}+Q_{22})+(8Q_{11}-8Q_{22}+42\gamma_{123})\cos 2\phi+(16Q_{12}+42\gamma_{223}+21\gamma_{333})\sin 2\phi)+42\sin^2\theta(-((4\gamma_{222}+3\gamma_{233})\cos 3\phi)+(4\gamma_{122}+\gamma_{133})\sin 3\phi) \right]. \quad (7)$$

The expressions of  $Z_1$ ,  $Z_2$ , and  $Z_3$  in point torque at  $O(\alpha)$  [eqn (44) in the paper] are obtained as

$$Z_1 = \frac{1}{16(2+\Gamma)(2+3\Gamma)} \left[ 5(4+8\Gamma+3\Gamma^2)(-Q_{22}\gamma_{122}-2Q_{23}\gamma_{123}+Q_{22}\gamma_{133}+Q_{11}(\gamma_{122}+2\gamma_{133})+2Q_{12}\gamma_{222}+2Q_{12}\gamma_{233})+Q_{13}(60+40\gamma_{223}+40\gamma_{333}+6\Gamma^2(4+5\gamma_{223}+5\gamma_{333})+8\Gamma(12+10\gamma_{223}+10\gamma_{333}-3\tau)-36\tau) \right], \quad (8)$$

$$Z_2 = -\frac{1}{16(2+\Gamma)(2+3\Gamma)} \left[ 5(4+8\Gamma+3\Gamma^2)(2Q_{12}\gamma_{122}+2Q_{13}\gamma_{123}-Q_{11}\gamma_{222}+Q_{22}\gamma_{222}-2Q_{11}\gamma_{233}-Q_{22}\gamma_{233})+Q_{23}(-60+40\gamma_{223}+80\Gamma\gamma_{223}+6\Gamma^2(-4+5\gamma_{223})+24\Gamma(-4+\tau)+36\tau) \right], \quad (9)$$

$$Z_3 = \frac{1}{16(2+\Gamma)(2+3\Gamma)} \left[ -10(4+8\Gamma+3\Gamma^2)(Q_{12}\gamma_{123} + Q_{13}\gamma_{133} + Q_{23}\gamma_{233}) + Q_{22}(-3\Gamma^2(8+5\gamma_{223} - 5\gamma_{333}) - 8\Gamma(12+5\gamma_{223}-5\gamma_{333}-3\tau) + 4(-15-5\gamma_{223}+5\gamma_{333}+9\tau)) + Q_{11}(3\Gamma^2(-8+5\gamma_{223} + 10\gamma_{333}) + 8\Gamma(-12+5\gamma_{223}+10\gamma_{333}+3\tau) + 4(-15+5\gamma_{223}+10\gamma_{333}+9\tau)) \right]. \quad (10)$$

## 2 Particle translating in the quadratic component of elliptical Poiseuille flow

The components of the disturbance velocity and the pressure fields in the fluid at the leading-order are obtained as

$$v_{d_{qe},r}^{(0)} = \frac{\mathcal{A}_1}{\xi} \cos \theta + \frac{1}{\xi^3} \left[ \mathcal{A}_2 + \mathcal{A}_3 \cos 2\theta + \mathcal{A}_4 \cos 2\phi \sin^2 \theta \right] \cos \theta - \frac{1}{14\xi^5} \left[ 5\mathcal{A}_3 \cos 3\theta + \cos \theta (3\mathcal{A}_3 + 10\mathcal{A}_4 \cos 2\phi \sin^2 \theta) \right], \quad (11)$$

$$v_{d_{qe},\theta}^{(0)} = -\frac{\mathcal{A}_1}{2\xi} \sin \theta + \frac{1}{56\xi^3} \left[ (56\mathcal{B}_1 - \mathcal{A}_4(13+7\cos 2\theta) \cos 2\phi) \sin \theta + 7\mathcal{A}_3 \sin 3\theta \right] + \frac{1}{112\xi^5} \left[ -(6\mathcal{A}_3 + 5\mathcal{A}_4 \cos 2\phi) \sin \theta + 15(-2\mathcal{A}_3 + \mathcal{A}_4 \cos 2\phi) \sin 3\theta \right], \quad (12)$$

$$v_{d_{qe},\phi}^{(0)} = \left[ \frac{1}{\xi^3} - \frac{1}{\xi^5} \right] \frac{5}{28} \mathcal{A}_4 \sin 2\theta \sin 2\phi, \quad (13)$$

and

$$p_{d_{qe}}^{(0)} = \frac{\mathcal{A}_1}{\xi^2} \cos \theta + \frac{1}{2\xi^4} \left[ \mathcal{A}_3(5\cos 2\theta - 1) + 5\mathcal{A}_4 \cos 2\phi \sin^2 \theta \right] \cos \theta, \quad (14)$$

respectively. The expressions for  $\mathcal{A}_1$ ,  $\mathcal{A}_2$ ,  $\mathcal{A}_3$ ,  $\mathcal{A}_4$ , and  $\mathcal{B}_1$  are given in eqn (27) and (28), respectively. The components of the displacement at  $O(\alpha)$  are obtained as

$$u_{d_{qe},r}^{(1)} = \frac{\mathcal{A}_1}{\xi} \cos \theta + \frac{\xi^2}{8} \left[ 8\mathcal{C}_1 - 5\mathcal{A}_3 \cos 2\theta - 5\mathcal{A}_4 \cos 2\phi \sin^2 \theta \right] \cos \theta - \frac{P_0 \xi}{2+3\Gamma}, \quad (15)$$

$$u_{d_{qe},\theta}^{(1)} = \frac{\mathcal{F}_1}{\xi} \sin \theta + \xi^2 \left[ \mathcal{F}_2 + \frac{5}{112} \mathcal{A}_4 (19 - 7\cos 2\theta) \cos 2\phi + \frac{5}{16} \mathcal{A}_3 \csc \theta \sin 3\theta \right] \sin \theta, \quad (16)$$

and

$$u_{d_{qe},\phi}^{(1)} = -\frac{15}{56} \xi^2 \mathcal{A}_4 \sin 2\theta \sin 2\phi. \quad (17)$$

The expressions for  $\mathcal{E}_1$ ,  $\mathcal{F}_1$  and  $\mathcal{F}_2$  are given in eqn (29) and (30), respectively. The components of disturbance velocity and the pressure fields in the fluid at  $O(\alpha)$  are obtained as

$$v_{d_{qe},r}^{(1)} = \frac{1}{\xi^2} \left[ \mathcal{H}_1 + \mathcal{H}_2 \cos 2\theta + \mathcal{H}_3 \cos 2\phi \sin^2 \theta \right] + \frac{1}{\xi^4} \left[ \mathcal{H}_4 + \mathcal{H}_5 \cos 2\theta + \mathcal{H}_6 \cos 4\theta + (\mathcal{H}_7 + \mathcal{H}_8 \cos 2\theta) \right. \\ \left. \times \cos 2\phi \sin^2 \theta + \mathcal{H}_9 \cos 4\phi \sin^4 \theta \right] + \frac{1}{\xi^6} \left[ \mathcal{H}_{10} + \mathcal{H}_{11} \cos 2\theta + \mathcal{H}_{12} \cos 4\theta + \mathcal{H}_{13} \cos 6\theta + (\mathcal{H}_{14} \right. \\ \left. + \mathcal{H}_{15} \cos 2\theta + \mathcal{H}_{16} \cos 4\theta) \cos 2\phi \sin^2 \theta + (\mathcal{H}_{17} + \mathcal{H}_{18} \cos 2\theta) \cos 4\phi \sin^4 \theta \right] + \frac{1}{924\xi^8} \left[ -4\mathcal{H}_{13} \right. \\ \left. \times (50 + 105 \cos 2\theta + 126 \cos 4\theta + 231 \cos 6\theta) - 28\mathcal{H}_{16}(35 + 60 \cos 2\theta + 33 \cos 4\theta) \cos 2\phi \sin^2 \theta \right. \\ \left. + 3773\mathcal{H}_9(9 + 11 \cos 2\theta) \cos 4\phi \sin^4 \theta \right] + P_0 \left[ \frac{1}{\xi} (\mathcal{H}_{19} \cos \theta) + \frac{1}{\xi^3} (\mathcal{H}_{20} \cos \theta + \mathcal{H}_{21} \cos \theta \cos 2\theta \right. \\ \left. + \mathcal{H}_{22} \cos \theta \cos 2\phi \sin^2 \theta) + \frac{1}{\xi^5} \left( \frac{1}{5} \mathcal{H}_{21} \cos \theta - \mathcal{H}_{21} \cos \theta \cos 2\theta - \mathcal{H}_{22} \cos \theta \cos 2\phi \sin^2 \theta \right) \right] \quad (18)$$

$$v_{d_{qe},\theta}^{(1)} = \frac{1}{\xi^4} \left[ \mathcal{J}_1 \cos \theta \cos 4\phi \sin^3 \theta + (\mathcal{J}_2 + \mathcal{J}_3 \cos 2\phi) \sin 2\theta + (\mathcal{J}_4 + \mathcal{J}_5 \cos 2\phi) \sin 4\theta \right] + \frac{1}{\xi^6} \left[ \mathcal{J}_6 \cos \theta \right. \\ \left. \times \cos 4\phi \sin^3 \theta + \mathcal{J}_7 \cos \theta \cos 2\theta \cos 4\phi \sin^3 \theta + \mathcal{J}_8 \sin 2\theta + \mathcal{J}_9 \cos 2\theta \sin 2\theta + \mathcal{J}_{10} \cos 4\theta \sin 2\theta \right. \\ \left. + \mathcal{J}_{11} \cos 2\phi \sin 2\theta + \mathcal{J}_{12} \cos 2\theta \cos 2\phi \sin 2\theta + \mathcal{J}_{13} \cos 4\theta \cos 2\phi \sin 2\theta \right] + \frac{1}{924\xi^8} \left[ -48\mathcal{H}_{13}(19 \right. \\ \left. + 12 \cos 2\theta + 33 \cos 4\theta) + 4\mathcal{H}_{16}(41 - 12 \cos 2\theta + 99 \cos 4\theta) \cos 2\phi - 539\mathcal{H}_9(7 + 33 \cos 2\theta) \right. \\ \left. \times \cos 4\phi \sin^2 \theta \right] \sin 2\theta + P_0 \left[ \frac{1}{\xi} \mathcal{J}_{14} \sin \theta + \frac{1}{\xi^3} (\mathcal{J}_{15} \sin \theta + \mathcal{J}_{16} \cos 2\theta \sin \theta + \mathcal{J}_{17} \cos 2\phi \sin \theta \right. \\ \left. + \mathcal{J}_{18} \cos 2\theta \cos 2\phi \sin \theta) - \frac{1}{65\xi^5} (39\mathcal{J}_{16}(3 + 5 \cos 2\theta) + 35\mathcal{J}_{17}(1 + 3 \cos 2\theta) \cos 2\phi) \sin \theta \right], \quad (19)$$

$$v_{d_{qe},\phi}^{(1)} = \frac{1}{\xi^4} \left[ (\mathcal{J}_1 + \mathcal{J}_2 \cos 2\theta) \sin \theta \sin 2\phi + \mathcal{J}_3 \sin^3 \theta \sin 4\phi \right] + \frac{1}{\xi^6} \left[ (\mathcal{J}_4 + \mathcal{J}_5 \cos 2\theta + \mathcal{J}_6 \cos 4\theta) \sin \theta \right. \\ \left. \times \sin 2\phi + (\mathcal{J}_7 + \mathcal{J}_8 \cos 2\theta) \sin^3 \theta \sin 4\phi \right] + \frac{1}{\xi^8} \left[ -\frac{2}{231} \mathcal{H}_{16}(35 + 60 \cos 2\theta + 33 \cos 4\theta) \sin \theta \right. \\ \left. \times \sin 2\phi + \frac{7}{3} \mathcal{H}_9(9 + 11 \cos 2\theta) \sin^3 \theta \sin 4\phi \right] + P_0 \left[ \frac{1}{4\xi^3} - \frac{7}{20\xi^5} \right] \mathcal{J}_9 \sin 2\theta \sin 2\phi, \quad (20)$$

and

$$p_{d_{qe}}^{(1)} = \frac{\mathcal{K}_1}{\xi^3} + \frac{1}{\xi^5} \left[ \mathcal{K}_2 + \mathcal{K}_3 \cos 2\theta + \mathcal{K}_4 \cos 4\theta + (\mathcal{K}_5 + \mathcal{K}_6 \cos 2\theta) \cos 2\phi \sin^2 \theta + \mathcal{K}_7 \cos 4\phi \sin^4 \theta \right] \\ + \frac{\mathcal{K}_8}{\xi^7} + P_0 \left[ \frac{1}{\xi^2} (\mathcal{K}_9 \cos \theta) + \frac{1}{\xi^4} (\mathcal{K}_{10} - 5\mathcal{K}_{10} \cos 2\theta + \mathcal{K}_{11} \cos 2\phi \sin^2 \theta) \cos \theta \right], \quad (21)$$

respectively. Here,

$$\mathcal{K}_1 = 2(\mathcal{H}_1 + \mathcal{H}_2 \cos 2\theta + \mathcal{H}_3 \cos 2\phi \sin^2 \theta) \quad (22)$$

$$\mathcal{K}_8 = -\frac{1}{294} [-4\mathcal{H}_{13}(50 + 105 \cos 2\theta + 126 \cos 4\theta + 231 \cos 6\theta) - 28\mathcal{H}_{16}(35 + 60 \cos 2\theta \\ + 33 \cos 4\theta) \cos 2\phi \sin^2 \theta + 3773\mathcal{H}_9(9 + 11 \cos 2\theta) \cos 4\phi \sin^4 \theta] \quad (23)$$

The expressions for  $\mathcal{H}_n$  (with  $n = 1, 2, \dots, 22$ ),  $\mathcal{J}_n$  (with  $n = 1, 2, \dots, 18$ ),  $\mathcal{I}_n$  (with  $n = 1, 2, \dots, 9$ ) and  $\mathcal{K}_n$  (with  $n = 2, 3, \dots, 7$  and  $9, 10, 11$ ) are given in eqn (31)-(69).

The components of the displacement at  $O(\alpha^2)$  are obtained as

$$\begin{aligned}
u_{qe,r}^{(2)} = & \frac{1}{270336(2+\Gamma)^2(2+3\Gamma)^2(14+17\Gamma)(14+19\Gamma)} \xi \left[ 152064(14+17\Gamma)(5+2\Gamma(4+\Gamma))(-336 \right. \\
& + \Gamma(-796-532\Gamma-97\Gamma^2+24(1+\Gamma)(2+3\Gamma)\xi^2)) + 3(-704(14+17\Gamma)(44576+\Gamma(133000 \\
& + \Gamma(148348+\Gamma(86978+9\Gamma(3279+523\Gamma)))))) + (2+3\Gamma)(-5408928+\Gamma(45241520 \\
& + \Gamma(203174800+\Gamma(265312840+\Gamma(133872038+22501155\Gamma)))))) \xi^2 + 47520(1+\Gamma)(2+\Gamma) \\
& \times (1+2\Gamma)(2+3\Gamma)^2(14+19\Gamma)\xi^4)(\psi_x^4+\psi_y^4) + 2(-704(14+17\Gamma)(158368+\Gamma(476440 \\
& + \Gamma(506164+3\Gamma(81298+9\Gamma(2099+223\Gamma)))))) - (2+3\Gamma)(21730464+\Gamma(49882960 \\
& + \Gamma(30285680+\Gamma(8254520+\Gamma(13803226+7705725\Gamma)))))) \xi^2 + 142560(1+\Gamma)(2+\Gamma) \\
& \times (1+2\Gamma)(2+3\Gamma)^2(14+19\Gamma)\xi^4)\psi_x^2\psi_y^2 + 792(-8(14+17\Gamma)(53536+\Gamma(188024+\Gamma(240828 \\
& + \Gamma(139922+\Gamma(37591+3984\Gamma)))))) + 3(2+3\Gamma)(-23072+\Gamma(29840+\Gamma(270784+\Gamma(380432 \\
& + \Gamma(187858+26243\Gamma)))))) \xi^2 + 540(1+\Gamma)(2+\Gamma)(1+2\Gamma)(2+3\Gamma)^2(14+19\Gamma)\xi^4)(\psi_x^2+\psi_y^2) \\
& + (2+3\Gamma)(12(12672(14+17\Gamma)(5+2\Gamma(4+\Gamma))(-112+\Gamma(-214-97\Gamma+72(1+\Gamma)\xi^2)) \\
& + (-528(14+17\Gamma)(8400+\Gamma(25196+\Gamma(25916+\Gamma(10919+1569\Gamma)))))) + (-3004960 \\
& + \Gamma(39545840+\Gamma(164058192+\Gamma(210758056+\Gamma(106120078+17932119\Gamma)))))) \xi^2 + 26400(1 \\
& + \Gamma)(2+\Gamma)(1+2\Gamma)(2+3\Gamma)(14+19\Gamma)\xi^4)(\psi_x^4+\psi_y^4) + 2(-176(14+17\Gamma)(14000+\Gamma(40388 \\
& + \Gamma(40148+9\Gamma(1773+223\Gamma)))) + (-4024160+\Gamma(-5046960+\Gamma(7610992+\Gamma(12918456 \\
& + (3637978-649731\Gamma)\Gamma)))) \xi^2 + 26400(1+\Gamma)(2+\Gamma)(1+2\Gamma)(2+3\Gamma)(14+19\Gamma)\xi^4)\psi_x^2\psi_y^2 \\
& + 88(-18(14+17\Gamma)(6160+\Gamma(19172+\Gamma(20872+83\Gamma(111+16\Gamma)))) + (-115360 \\
& + \Gamma(415760+\Gamma(2270304+\Gamma(3009952+\Gamma(1480306+215943\Gamma)))))) \xi^2 + 900(1+\Gamma)(2+\Gamma) \\
& \times (1+2\Gamma)(2+3\Gamma)(14+19\Gamma)\xi^4)(\psi_x^2+\psi_y^2)) \cos 2\theta + 105(2+\Gamma)(2+3\Gamma)(14+19\Gamma)\xi^2 \\
& \times ((-10732-21264\Gamma-10589\Gamma^2+5280(1+\Gamma)(1+2\Gamma)\xi^2)\psi_x^4 + 2(-14372-27504\Gamma-12799\Gamma^2 \\
& + 5280(1+\Gamma)(1+2\Gamma)\xi^2)\psi_x^2\psi_y^2 + (-10732-21264\Gamma-10589\Gamma^2+5280(1+\Gamma)(1+2\Gamma)\xi^2)\psi_y^4 \\
& + 88(-412-804\Gamma-389\Gamma^2+180(1+\Gamma)(1+2\Gamma)\xi^2)(\psi_x^2+\psi_y^2)) \cos 4\theta - 80(2+\Gamma)(\psi_x^2-\psi_y^2) \\
& \times (66(12(14+17\Gamma)(168+\Gamma(470+337\Gamma)) - (2+3\Gamma)(28840+\Gamma(75932+\Gamma(67178 \\
& + 21451\Gamma)))) \xi^2 + 900(1+\Gamma)(1+2\Gamma)(2+3\Gamma)(14+19\Gamma)\xi^4) + (-88(14+17\Gamma)(616+\Gamma(4010 \\
& + 3\Gamma(1943+735\Gamma))) + (2+3\Gamma)(-503160+\Gamma(-207644+\Gamma(723654+279563\Gamma)))) \xi^2 \\
& + 19800(1+\Gamma)(1+2\Gamma)(2+3\Gamma)(14+19\Gamma)\xi^4)(\psi_x^2+\psi_y^2) + 21(2+3\Gamma)(14+19\Gamma)\xi^2(22(-412 \\
& - 804\Gamma-389\Gamma^2+180(1+\Gamma)(1+2\Gamma)\xi^2) + (-2396-4824\Gamma-2473\Gamma^2+1320(1+\Gamma)(1 \\
& + 2\Gamma)\xi^2)(\psi_x^2+\psi_y^2)) \cos 2\theta \cos 2\phi \sin^2 \theta + 34440(2+\Gamma)^2(2+3\Gamma)(14+17\Gamma)(14+19\Gamma)\xi^2 \\
& \times (\psi_x-\psi_y)^2(\psi_x+\psi_y)^2 \cos 4\phi \sin^4 \theta \left. \right] - P_0 \left[ \frac{3}{2(2+\Gamma)(2+3\Gamma)^2\xi} ((4+8\Gamma+3\Gamma^2 \right. \\
& \left. + 2(-1+\Gamma^2)\xi^3) + (2+\Gamma)(2+3\Gamma)(\psi_x^2+\psi_y^2)) \cos \theta \right], \tag{24}
\end{aligned}$$

$$\begin{aligned}
u_{qe,\theta}^{(2)} = & \frac{1}{135168} \xi \left[ 17220 \xi^2 (\psi_x^2 - \psi_y^2)^2 \cos \theta \cos 4\phi \sin^3 \theta + \frac{1}{(2+\Gamma)^2(2+3\Gamma)(14+17\Gamma)(14+19\Gamma)} \right. \\
& \times \left[ -76032(14+17\Gamma)(5+2\Gamma(4+\Gamma))(-112-214\Gamma-97\Gamma^2+24(1+\Gamma)(7+5\Gamma)\xi^2) \right. \\
& -9(-352(14+17\Gamma)(8400+\Gamma(25196+\Gamma(25916+\Gamma(10919+1569\Gamma)))) + (85468320 \\
& +\Gamma(363516752+\Gamma(588408176+\Gamma(450819128+3\Gamma(54400798+7423935\Gamma)))))\xi^2 \\
& +3520(1+\Gamma)(2+\Gamma)(2+3\Gamma)(9+7\Gamma)(14+19\Gamma)\xi^4)(\psi_x^4 + \psi_y^4) - 2(-1056(14+17\Gamma) \\
& \times (14000+\Gamma(40388+\Gamma(40148+9\Gamma(1773+223\Gamma)))) + (214221280+\Gamma(811856368 \\
& +\Gamma(1159899984+\Gamma(763309352+\Gamma(220127246+19036695\Gamma)))))\xi^2 + 31680(1+\Gamma) \\
& \times (2+\Gamma)(2+3\Gamma)(9+7\Gamma)(14+19\Gamma)\xi^4)\psi_x^2\psi_y^2 - 264(-36(14+17\Gamma)(6160+\Gamma(19172 \\
& +\Gamma(20872+83\Gamma(111+16\Gamma)))) + (4682720+\Gamma(19309712+\Gamma(30458016+\Gamma(22718368 \\
& +\Gamma(7874554+978495\Gamma)))))\xi^2 + 360(1+\Gamma)(2+\Gamma)(2+3\Gamma)(9+7\Gamma)(14+19\Gamma)\xi^4)(\psi_x^2 \\
& +\psi_y^2) + 5(2+\Gamma)(4(\psi_x^2 - \psi_y^2)(66(-12(14+17\Gamma)(168+\Gamma(470+337\Gamma)) - (2+3\Gamma)(78680 \\
& +\Gamma(220852+\Gamma(198118+55841\Gamma))))\xi^2 + 72(1+\Gamma)(2+3\Gamma)(9+7\Gamma)(14+19\Gamma)\xi^4) \\
& + (88(14+17\Gamma)(616+\Gamma(4010+3\Gamma(1943+735\Gamma))) - 3(2+3\Gamma)(2465512+\Gamma(6890292 \\
& +\Gamma(6085022+1643967\Gamma))))\xi^2 + 1584(1+\Gamma)(2+3\Gamma)(9+7\Gamma)(14+19\Gamma)\xi^4)(\psi_x^2 + \psi_y^2)) \cos 2\phi \\
& + 21(2+3\Gamma)(14+19\Gamma)\xi^2 \cos 2\theta ((10732+21264\Gamma+10589\Gamma^2-2112(1+\Gamma)(9+7\Gamma)\xi^2) \\
& \times (\psi_x^4 + \psi_y^4) + 2(14372+27504\Gamma+12799\Gamma^2-2112(1+\Gamma)(9+7\Gamma)\xi^2)\psi_x^2\psi_y^2 - 88(-412 \\
& -804\Gamma-389\Gamma^2+72(1+\Gamma)(9+7\Gamma)\xi^2)(\psi_x^2 + \psi_y^2) - 4(\psi_x^2 - \psi_y^2)(22(-412-804\Gamma-389\Gamma^2 \\
& +72(1+\Gamma)(9+7\Gamma)\xi^2) + (-2396-4824\Gamma-2473\Gamma^2+528(1+\Gamma)(9+7\Gamma)\xi^2)(\psi_x^2 + \psi_y^2)) \\
& \times \cos 2\phi) \Big] \sin 2\theta \Big] + P_0 \left[ \frac{3}{4(2+\Gamma)(2+3\Gamma)^2\xi} ((6+11\Gamma+3\Gamma^2+4(1+\Gamma)(3+2\Gamma)\xi^3) \right. \\
& \left. + (3+\Gamma)(2+3\Gamma)(\psi_x^2 + \psi_y^2)) \sin \theta \right], \tag{25}
\end{aligned}$$

$$\begin{aligned}
u_{qe,\phi}^{(2)} = & \frac{1}{33792(2+\Gamma)(2+3\Gamma)(14+17\Gamma)(14+19\Gamma)} 5\xi (\psi_x^2 - \psi_y^2) \sin \theta \left[ (132(12(14+17\Gamma)(168+\Gamma(470 \right. \\
& +337\Gamma)) + (2+3\Gamma)(37912+\Gamma(90848+\Gamma(65216+13015\Gamma))))\xi^2 + 180(1+\Gamma)(2+3\Gamma)(9+7\Gamma) \\
& \times (14+19\Gamma)\xi^4) + (-176(14+17\Gamma)(616+\Gamma(4010+3\Gamma(1943+735\Gamma))) + (2+3\Gamma)(8353688 \\
& +\Gamma(21352972+\Gamma(17033794+4151585\Gamma))))\xi^2 + 7920(1+\Gamma)(2+3\Gamma)(9+7\Gamma)(14+19\Gamma)\xi^4) \\
& \times (\psi_x^2 + \psi_y^2) + 7(2+3\Gamma)(14+19\Gamma)\xi^2(132(4-42\Gamma-67\Gamma^2+36(1+\Gamma)(9+7\Gamma)\xi^2) + (51332 \\
& +85848\Gamma+28111\Gamma^2+1584(1+\Gamma)(9+7\Gamma)\xi^2)(\psi_x^2 + \psi_y^2)) \cos 2\theta \sin 2\phi - 861(2+\Gamma) \\
& \left. \times (2+3\Gamma)(14+17\Gamma)(14+19\Gamma)\xi^2(\psi_x^2 - \psi_y^2) \sin^2 \theta \sin 4\phi \right]. \tag{26}
\end{aligned}$$

The expressions of  $\mathcal{A}_n, \mathcal{B}_n, \mathcal{C}_n, \mathcal{F}_n, \mathcal{H}_n, \mathcal{I}_n, \mathcal{J}_n$ , and  $\mathcal{K}_n$  in velocity, pressure, displacement and deformation till  $O(\alpha)$  are obtained as

$$\mathcal{A}_1 = \frac{3 + \psi_x^2 + \psi_y^2}{2}, \mathcal{A}_2 = -\frac{4 + \psi_x^2 + \psi_y^2}{8}, \mathcal{A}_3 = -\frac{7(\psi_x^2 + \psi_y^2)}{8}, \mathcal{A}_4 = \frac{7(\psi_x^2 - \psi_y^2)}{4}, \tag{27}$$

$$\mathcal{B}_1 = -\frac{1}{4} - \frac{11(\psi_x^2 + \psi_y^2)}{64}, \quad (28)$$

$$\mathcal{E}_1 = -\frac{3[32(-1 + \Gamma^2) + (-44 + 40\Gamma + 39\Gamma^2)(\psi_x^2 + \psi_y^2)]}{64(2 + \Gamma)(2 + 3\Gamma)}, \quad \mathcal{F}_1 = -\frac{3 + \Gamma}{4 + 2\Gamma}\mathcal{A}_1, \quad (29)$$

$$\mathcal{F}_2 = \frac{192(3 + 5\Gamma + 2\Gamma^2) + (932 + 1160\Gamma + 363\Gamma^2)(\psi_x^2 + \psi_y^2)}{128(2 + \Gamma)(2 + 3\Gamma)}, \quad (30)$$

$$\mathcal{H}_1 = \frac{1}{384(2 + \Gamma)(2 + 3\Gamma)} [216(5 + 2\Gamma(4 + \Gamma)) + 9(100 + \Gamma(88 + 7\Gamma))(\psi_x^2 + \psi_y^2) + 4[-3(10 + \Gamma(44 + 21\Gamma))\psi_x^4 + 4(35 + 34\Gamma + 6\Gamma^2)\psi_x^2\psi_y^2 - 3(10 + \Gamma(44 + 21\Gamma))\psi_y^4]], \quad (31)$$

$$\mathcal{H}_2 = 3\mathcal{H}_1, \quad \mathcal{H}_3 = \frac{5(\psi_x^2 - \psi_y^2)(9 + 8(\psi_x^2 + \psi_y^2))}{192}, \quad (32)$$

$$\mathcal{H}_4 = \frac{1}{135168(2 + \Gamma)(2 + 3\Gamma)} [-76032(5 + 2\Gamma(4 + \Gamma)) + 3(-13100 + \Gamma(102632 + 62643\Gamma))\psi_x^4 - 2(347500 + \Gamma(308504 + 43221\Gamma))\psi_x^2\psi_y^2 + 3(-13100 + \Gamma(102632 + 62643\Gamma))\psi_y^4 - 396(1520 + \Gamma(1784 + 281\Gamma))(\psi_x^2 + \psi_y^2)], \quad (33)$$

$$\mathcal{H}_5 = \frac{1}{11264(2 + \Gamma)(2 + 3\Gamma)} [-19008(5 + 2\Gamma(4 + \Gamma)) + (-4540 + \Gamma(69064 + 40551\Gamma))\psi_x^4 - 6(23580 + \Gamma(21112 + 3033\Gamma))\psi_x^2\psi_y^2 + (-4540 + \Gamma(69064 + 40551\Gamma))\psi_y^4 - 132(1000 + \Gamma(1128 + 167\Gamma))(\psi_x^2 + \psi_y^2)], \quad (34)$$

$$\mathcal{H}_6 = \frac{1}{45056(2 + \Gamma)(2 + 3\Gamma)} [175((-604 + \Gamma(904 + 735\Gamma))\psi_x^4 - 2(1844 + \Gamma(1576 + 195\Gamma))\psi_x^2\psi_y^2 + (-604 + \Gamma(904 + 735\Gamma))\psi_y^4 - 132(4 + \Gamma)(4 + 5\Gamma)(\psi_x^2 + \psi_y^2))], \quad (35)$$

$$\mathcal{H}_7 = \frac{1}{8448(2 + \Gamma)(2 + 3\Gamma)} [5(\psi_x^2 - \psi_y^2)(99(384 + \Gamma(568 + 113\Gamma)) - 2(-4846 + \Gamma(10108 + 7503\Gamma))) \times (\psi_x^2 + \psi_y^2)], \quad (36)$$

$$\mathcal{H}_8 = \frac{175(\psi_x^2 - \psi_y^2)(33(4 + \Gamma)(4 + 5\Gamma) - 2(-74 + \Gamma(116 + 93\Gamma))(\psi_x^2 + \psi_y^2))}{2816(2 + \Gamma)(2 + 3\Gamma)}, \quad (37)$$

$$\mathcal{H}_9 = \frac{525(\psi_x^2 - \psi_y^2)^2}{5632}, \quad \mathcal{H}_{10} = \frac{1}{540672(2 + \Gamma)(2 + 3\Gamma)} [5(-3(2756 + \Gamma(81544 + 44835\Gamma))\psi_x^4 + 2(174652 + \Gamma(121208 + 2685\Gamma))\psi_x^2\psi_y^2 - 3(2756 + \Gamma(81544 + 44835\Gamma))\psi_y^4 + 14256(4 + \Gamma) \times (4 + 5\Gamma)(\psi_x^2 + \psi_y^2))], \quad (38)$$

$$\mathcal{H}_{11} = \frac{1}{360448(2 + \Gamma)(2 + 3\Gamma)} [25(-(1252 + \Gamma(70088 + 38955\Gamma))\psi_x^4 + 2(52148 + \Gamma(36712 + 1095\Gamma))\psi_x^2\psi_y^2 - (1252 + \Gamma(70088 + 38955\Gamma))\psi_y^4 + 4224(4 + \Gamma)(4 + 5\Gamma)(\psi_x^2 + \psi_y^2))], \quad (39)$$

$$\mathcal{H}_{12} = \frac{1}{180224(2 + \Gamma)(2 + 3\Gamma)} [175((652 - \Gamma(7144 + 4263\Gamma))\psi_x^4 + 2(6788 + \Gamma(5128 + 339\Gamma))\psi_x^2\psi_y^2 + (652 - \Gamma(7144 + 4263\Gamma))\psi_y^4 + 528(4 + \Gamma)(4 + 5\Gamma)(\psi_x^2 + \psi_y^2))], \quad (40)$$

$$\mathcal{H}_{13} = -\frac{8575(3\psi_x^4 + 2\psi_x^2\psi_y^2 + 3\psi_y^4)}{32768}, \quad (41)$$

$$\mathcal{H}_{14} = \frac{1}{67584(2+\Gamma)(2+3\Gamma)} [125(\psi_x^2 - \psi_y^2)(-792(4+\Gamma)(4+5\Gamma) + (6052 + \Gamma(24776 + 11667\Gamma))) \times (\psi_x^2 + \psi_y^2)], \quad (42)$$

$$\mathcal{H}_{15} = \frac{525(\psi_x^2 - \psi_y^2)(-22(4+\Gamma)(4+5\Gamma) + (228 + \Gamma(808 + 369\Gamma))(\psi_x^2 + \psi_y^2))}{5632(2+\Gamma)(2+3\Gamma)}, \quad (43)$$

$$\mathcal{H}_{16} = \frac{8575(\psi_x^4 - \psi_y^4)}{2048}, \mathcal{H}_{17} = -\frac{151}{4}\mathcal{H}_9, \mathcal{H}_{18} = -\frac{539}{12}\mathcal{H}_9, \mathcal{H}_{19} = -\frac{3(1 + \psi_x^2 + \psi_y^2)}{2(2+3\Gamma)}, \quad (44)$$

$$\mathcal{H}_{20} = \frac{12 + 5\psi_x^2 + 5\psi_y^2}{16 + 24\Gamma}, \mathcal{H}_{21} = \frac{35(\psi_x^2 + \psi_y^2)}{8(2+3\Gamma)}, \mathcal{H}_{22} = \frac{35(-\psi_x^2 + \psi_y^2)}{4(2+3\Gamma)}, \quad (45)$$

$$\mathcal{I}_1 = -\frac{2}{5}\mathcal{H}_9, \quad (46)$$

$$\mathcal{I}_2 = \frac{1}{33792(2+\Gamma)(2+3\Gamma)} [-38016(5 + 2\Gamma(4+\Gamma)) + 9(1340 + 3\Gamma(3944 + 2051\Gamma))\psi_x^4 - 2(76940 + \Gamma(71512 + 11373\Gamma))\psi_x^2\psi_y^2 + 9(1340 + 3\Gamma(3944 + 2051\Gamma))\psi_y^4 - 396(480 + \Gamma(472 + 53\Gamma)) \times (\psi_x^2 + \psi_y^2)], \quad (47)$$

$$\mathcal{I}_3 = \frac{5(\psi_x^2 - \psi_y^2)(99\Gamma(8 + 7\Gamma) + 4(199 + 794\Gamma + 372\Gamma^2)(\psi_x^2 + \psi_y^2))}{8448(2+\Gamma)(2+3\Gamma)}, \quad (48)$$

$$\mathcal{I}_4 = \frac{1}{22528(2+\Gamma)(2+3\Gamma)} [35((-604 + \Gamma(904 + 735\Gamma))\psi_x^4 - 2(1844 + \Gamma(1576 + 195\Gamma))\psi_x^2\psi_y^2 + (-604 + \Gamma(904 + 735\Gamma))\psi_y^4 - 132(4+\Gamma)(4+5\Gamma)(\psi_x^2 + \psi_y^2))], \quad (49)$$

$$\mathcal{I}_5 = \frac{35(\psi_x^2 - \psi_y^2)(-33(4+\Gamma)(4+5\Gamma) + 2(-74 + \Gamma(116 + 93\Gamma))(\psi_x^2 + \psi_y^2))}{5632(2+\Gamma)(2+3\Gamma)}, \quad (50)$$

$$\mathcal{I}_6 = \frac{211}{15}\mathcal{H}_9, \mathcal{I}_7 = \frac{77}{3}\mathcal{H}_9, \quad (51)$$

$$\mathcal{I}_8 = \frac{1}{135168(2+\Gamma)(2+3\Gamma)} [5(-9(4596 + \Gamma(14824 + 6615\Gamma))\psi_x^4 + 2(25636 + (584 - 9285\Gamma)\Gamma) \times \psi_x^2\psi_y^2 - 9(4596 + \Gamma(14824 + 6615\Gamma))\psi_y^4 + 3168(4+\Gamma)(4+5\Gamma)(\psi_x^2 + \psi_y^2))], \quad (52)$$

$$\mathcal{I}_9 = \frac{1}{11264(2+\Gamma)(2+3\Gamma)} [35((788 - \Gamma(2648 + 1785\Gamma))\psi_x^4 + 2(3548 + \Gamma(2872 + 285\Gamma))\psi_x^2\psi_y^2 + (788 - \Gamma(2648 + 1785\Gamma))\psi_y^4 + 264(4+\Gamma)(4+5\Gamma)(\psi_x^2 + \psi_y^2))], \quad (53)$$

$$\mathcal{I}_{10} = \frac{8}{7}\mathcal{H}_{13}, \quad (54)$$

$$\mathcal{I}_{11} = -\frac{5(\psi_x^2 - \psi_y^2)(264(4+\Gamma)(4+5\Gamma) + (6196 + \Gamma(8168 + 2271\Gamma))(\psi_x^2 + \psi_y^2))}{11264(2+\Gamma)(2+3\Gamma)}, \quad (55)$$

$$\mathcal{I}_{12} = \frac{35(\psi_x^2 - \psi_y^2)(66(4+\Gamma)(4+5\Gamma) - (-284 + \Gamma(488 + 381\Gamma))(\psi_x^2 + \psi_y^2))}{2816(2+\Gamma)(2+3\Gamma)}, \quad (56)$$

$$\mathcal{I}_{13} = -\frac{2}{7}\mathcal{H}_{16}, \mathcal{I}_{14} = \frac{3(1 + \psi_x^2 + \psi_y^2)}{4(2+3\Gamma)}, \mathcal{I}_{15} = \frac{24 + 45\psi_x^2 + 45\psi_y^2}{32(2+3\Gamma)}, \quad (57)$$

$$\mathcal{I}_{16} = \frac{35(\psi_x^2 + \psi_y^2)}{32(2+3\Gamma)}, \mathcal{I}_{17} = \frac{65(\psi_x^2 - \psi_y^2)}{32(2+3\Gamma)}, \mathcal{I}_{18} = \frac{7}{13}\mathcal{I}_{17}, \quad (58)$$



$$\mathcal{J}_1 = \frac{5(\psi_x^2 - \psi_y^2)(198(40 + \Gamma(56 + 9\Gamma)) - (-1340 + \Gamma(6824 + 4341\Gamma))(\psi_x^2 + \psi_y^2))}{8448(2 + \Gamma)(2 + 3\Gamma)}, \quad (59)$$

$$\mathcal{J}_2 = \frac{5(\psi_x^2 - \psi_y^2)(198(72 + \Gamma(104 + 19\Gamma)) - (-3284 + \Gamma(9272 + 6447\Gamma))(\psi_x^2 + \psi_y^2))}{8448(2 + \Gamma)(2 + 3\Gamma)}, \quad (60)$$

$$\mathcal{J}_3 = \frac{2}{5}\mathcal{H}_9, \quad (61)$$

$$\mathcal{J}_4 = \frac{25(\psi_x^2 - \psi_y^2)(-396(4 + \Gamma)(4 + 5\Gamma) + (716 + \Gamma(7768 + 4101\Gamma))(\psi_x^2 + \psi_y^2))}{16896(2 + \Gamma)(2 + 3\Gamma)}, \quad (62)$$

$$\mathcal{J}_5 = \frac{35(\psi_x^2 - \psi_y^2)(-99(4 + \Gamma)(4 + 5\Gamma) + (344 + \Gamma(2272 + 1149\Gamma))(\psi_x^2 + \psi_y^2))}{4224(2 + \Gamma)(2 + 3\Gamma)}, \quad (63)$$

$$\mathcal{J}_6 = \frac{12}{49}\mathcal{H}_{16}, \mathcal{J}_7 = -\frac{266}{15}\mathcal{H}_9, \mathcal{J}_8 = -22\mathcal{H}_9, \mathcal{J}_9 = \frac{25(-\psi_x^2 + \psi_y^2)}{4(2 + 3\Gamma)}, \quad (64)$$

$$\mathcal{K}_2 = \frac{1}{22528(2 + \Gamma)(2 + 3\Gamma)} [63((-604 + \Gamma(904 + 735\Gamma))\psi_x^4 - 2(1844 + \Gamma(1576 + 195\Gamma))\psi_x^2\psi_y^2 + (-604 + \Gamma(904 + 735\Gamma))\psi_y^4 - 132(4 + \Gamma)(4 + 5\Gamma)(\psi_x^2 + \psi_y^2))], \quad (65)$$

$$\mathcal{K}_3 = \frac{20}{9}\mathcal{K}_2, \mathcal{K}_4 = \frac{35}{9}\mathcal{K}_2, \quad (66)$$

$$\mathcal{K}_5 = \frac{175(\psi_x^2 - \psi_y^2)(33(4 + \Gamma)(4 + 5\Gamma) - 2(-74 + \Gamma(116 + 93\Gamma))(\psi_x^2 + \psi_y^2))}{1408(2 + \Gamma)(2 + 3\Gamma)}, \quad (67)$$

$$\mathcal{K}_6 = \frac{7}{5}\mathcal{K}_5, \mathcal{K}_7 = \frac{14}{5}\mathcal{H}_9, \mathcal{K}_9 = -\frac{3(1 + \psi_x^2 + \psi_y^2)}{2(2 + 3\Gamma)}, \mathcal{K}_{10} = -\frac{35(\psi_x^2 + \psi_y^2)}{16(2 + 3\Gamma)}, \quad (68)$$

$$\mathcal{K}_{11} = -\frac{175(\psi_x^2 - \psi_y^2)}{8(2 + 3\Gamma)}. \quad (69)$$

The expressions of  $\mathcal{L}_n$  in the surface deformation at  $O(\alpha^2)$  are obtained as

$$\begin{aligned} \mathcal{L}_1 = & -\frac{1}{2162688(2 + \Gamma)^2(2 + 3\Gamma)^2(14 + 17\Gamma)(14 + 19\Gamma)} [304128(14 + 17\Gamma)(7840 \\ & + \Gamma(33504 + \Gamma(53806 + \Gamma(40067 + \Gamma(13704 + 1739\Gamma)))) + 3(3828969536 + \Gamma(19657251968 \\ & + \Gamma(40731330192 + \Gamma(43445669056 + \Gamma(25023158572 + 9\Gamma(813558984 + 94192115\Gamma))))))\psi_x^4 \\ & + 2(8793555008 + \Gamma(39493764224 + \Gamma(66758503056 + \Gamma(50939754688 + \Gamma(14952492076 \\ & - 3\Gamma(246275624 + 268856295\Gamma))))))\psi_x^2\psi_y^2 + 3(3828969536 + \Gamma(19657251968 \\ & + \Gamma(40731330192 + \Gamma(43445669056 + \Gamma(25023158572 + 9\Gamma(813558984 + 94192115\Gamma))))))\psi_y^4 \\ & + 6336(5509504 + \Gamma(27914608 + \Gamma(56856960 + \Gamma(59270984 + \Gamma(33048488 \\ & + 9208023\Gamma + 992088\Gamma^2)))))(\psi_x^2 + \psi_y^2)], \end{aligned} \quad (70)$$

$$\mathcal{L}_2 = \frac{1}{1441792(2+\Gamma)^2(2+3\Gamma)^2(14+17\Gamma)(14+19\Gamma)} [202752(14+17\Gamma)(5600+\Gamma(27360+\Gamma(50066+\Gamma(42109+\Gamma(15864+2101\Gamma)))))) - (2634134720+\Gamma(10174509440+\Gamma(21446075568+\Gamma(34750482496+\Gamma(35446691908+3\Gamma(5917712968+1100401563\Gamma))))))\psi_x^4 + 6(-598261440+\Gamma(970209920+\Gamma(10885313744+\Gamma(21189560768+21\Gamma(831256684+308613192\Gamma+42016347\Gamma^2))))))\psi_x^2\psi_y^2 - (2634134720+\Gamma(10174509440+\Gamma(21446075568+\Gamma(34750482496+\Gamma(35446691908+3\Gamma(5917712968+1100401563\Gamma))))))\psi_y^4 + 5632(2481920+\Gamma(15231920+\Gamma(36584256+\Gamma(43640392+\Gamma(26832856+7843683\Gamma+812898\Gamma^2)))))(\psi_x^2+\psi_y^2)] , \quad (71)$$

$$\mathcal{L}_3 = -\frac{5}{720896(2+\Gamma)(2+3\Gamma)(14+17\Gamma)} [(-477848+\Gamma(3199164+\Gamma(6842534+2783505\Gamma)))\psi_x^4 + 2(-2774408+\Gamma(-4182636+\Gamma(-457246+691995\Gamma)))\psi_x^2\psi_y^2 + (-477848+\Gamma(3199164+\Gamma(6842534+2783505\Gamma)))\psi_y^4 + 4928(-208+\Gamma(-306+\Gamma(109+240\Gamma)))(\psi_x^2+\psi_y^2)] , \quad (72)$$

$$\mathcal{L}_4 = -\frac{5}{28}\mathcal{H}_{13}, \mathcal{L}_5 = \frac{1}{270336(2+\Gamma)(2+3\Gamma)(14+17\Gamma)(14+19\Gamma)} [5(\psi_x^2-\psi_y^2)(1056(61600+\Gamma(246476+\Gamma(360128+\Gamma(219889+43092\Gamma)))) + (145457200+\Gamma(459208832+\Gamma(473450696+\Gamma(169213408+13223499\Gamma)))))(\psi_x^2+\psi_y^2)] , \quad (73)$$

$$\mathcal{L}_6 = -\frac{1}{22528(2+\Gamma)(2+3\Gamma)(14+17\Gamma)} [35(\psi_x^2-\psi_y^2)(88(-208+\Gamma(-306+\Gamma(109+240\Gamma)))) + 3(-10888+\Gamma(-6812+3\Gamma(5054+3081\Gamma)))(\psi_x^2+\psi_y^2)] , \quad (74)$$

$$\mathcal{L}_7 = \frac{5}{28}\mathcal{H}_{16}, \mathcal{L}_8 = -\frac{2819}{1680}\mathcal{H}_9, \mathcal{L}_9 = \frac{385}{48}\mathcal{H}_9, \mathcal{L}_{10} = \frac{1}{(2+3\Gamma)^2}, \mathcal{L}_{11} = -\frac{105(\psi_x^2+\psi_y^2)}{128(2+3\Gamma)}, \quad (75)$$

$$\mathcal{L}_{12} = -\frac{3(64(5+8\Gamma+2\Gamma^2)+3(220+184\Gamma+21\Gamma^2)(\psi_x^2+\psi_y^2))}{128(2+\Gamma)(2+3\Gamma)^2}, \mathcal{L}_{13} = \frac{105(\psi_x^2-\psi_y^2)}{32(2+3\Gamma)}. \quad (76)$$

The expressions of  $\mathcal{X}_n$  in the point force till  $O(\alpha^2)$  are obtained as

$$\mathcal{X}_1 = \frac{9(-140-360\Gamma-227\Gamma^2+6\Gamma^3+\Gamma^4)}{8(2+\Gamma)(2+3\Gamma)^2(14+19\Gamma)}, \mathcal{X}_2 = \frac{3(-2520-4244\Gamma+234\Gamma^2+1893\Gamma^3+47\Gamma^4)}{32(2+\Gamma)(2+3\Gamma)^2(14+19\Gamma)}, \quad (77)$$

$$\mathcal{X}_3 = -\frac{3047408+14243936\Gamma+27918120\Gamma^2+29116864\Gamma^3+15872575\Gamma^4+3404742\Gamma^5}{448(2+\Gamma)(2+3\Gamma)^2(14+17\Gamma)(14+19\Gamma)}, \quad (78)$$

$$\mathcal{X}_4 = -\frac{142225832+608291292\Gamma+980502694\Gamma^2+715141569\Gamma^3+202539888\Gamma^4}{44352(2+3\Gamma)^2(14+17\Gamma)(14+19\Gamma)}, \quad (79)$$

$$\mathcal{X}_5 = \frac{-26025272-48717452\Gamma+21169226\Gamma^2+75027291\Gamma^3+29247957\Gamma^4}{14784(2+3\Gamma)^2(14+17\Gamma)(14+19\Gamma)}, \quad (80)$$

$$\mathcal{X}_6 = \frac{-4220272+14434336\Gamma+92547880\Gamma^2+140403704\Gamma^3+82322565\Gamma^4+16118532\Gamma^5}{2016(2+\Gamma)(2+3\Gamma)^2(14+17\Gamma)(14+19\Gamma)}. \quad (81)$$

### 3 Particle translating in the quadratic component of Plane Poiseuille flow

The expressions of  $A_n, B_n, E_n, F_n, H_n, I_n, J_n, K_n$ , and  $L_n$  in velocity, pressure, displacement, deformation and point force at different orders in  $\alpha$  are obtained as

$$A_1 = \frac{3 + \psi^2}{2}, A_2 = -\frac{4 + \psi^2}{8}, A_3 = -\frac{7\psi^2}{8}, A_4 = \frac{7\psi^2}{4}, B_1 = \left(-\frac{1}{4} - \frac{11\psi^2}{64}\right), \quad (82)$$

$$E_1 = -\frac{3(32(-1 + \Gamma^2) + (-2 + 3\Gamma)(22 + 13\Gamma)\psi^2)}{64(2 + \Gamma)(2 + 3\Gamma)}, F_1 = -\frac{(3 + \Gamma)(3 + \psi^2)}{4(2 + \Gamma)}, \quad (83)$$

$$F_2 = \frac{192(1 + \Gamma)(3 + 2\Gamma) + (932 + \Gamma(1160 + 363\Gamma))\psi^2}{128(2 + \Gamma)(2 + 3\Gamma)}, \quad (84)$$

$$H_1 = \frac{72(5 + 2\Gamma(4 + \Gamma)) + 3(100 + \Gamma(88 + 7\Gamma))\psi^2 - 4(10 + \Gamma(44 + 21\Gamma))\psi^4}{128(2 + \Gamma)(2 + 3\Gamma)}, \quad (85)$$

$$H_2 = 3H_1, H_3 = \frac{5(9\psi^2 + 8\psi^4)}{192}, \quad (86)$$

$$H_4 = \frac{1}{45056(2 + \Gamma)(2 + 3\Gamma)} \left[ -25344(5 + 2\Gamma(4 + \Gamma)) - 132(1520 + \Gamma(1784 + 281\Gamma))\psi^2 + (-13100 + \Gamma(102632 + 62643\Gamma))\psi^4 \right], \quad (87)$$

$$H_5 = \frac{1}{11264(2 + \Gamma)(2 + 3\Gamma)} \left[ -19008(5 + 2\Gamma(4 + \Gamma)) - 132(1000 + \Gamma(1128 + 167\Gamma))\psi^2 + (-4540 + \Gamma(69064 + 40551\Gamma))\psi^4 \right], \quad (88)$$

$$H_6 = \frac{175(-132(4 + \Gamma)(4 + 5\Gamma)\psi^2 + (-604 + \Gamma(904 + 735\Gamma))\psi^4)}{45056(2 + \Gamma)(2 + 3\Gamma)}, \quad (89)$$

$$H_7 = \frac{5\psi^2(99(384 + \Gamma(568 + 113\Gamma)) - 2(-4846 + \Gamma(10108 + 7503\Gamma))\psi^2)}{8448(2 + \Gamma)(2 + 3\Gamma)}, \quad (90)$$

$$H_8 = \frac{175\psi^2(33(4 + \Gamma)(4 + 5\Gamma) - 2(-74 + \Gamma(116 + 93\Gamma))\psi^2)}{2816(2 + \Gamma)(2 + 3\Gamma)}, \quad (91)$$

$$H_9 = \frac{525\psi^4}{5632}, H_{10} = \frac{5(14256(4 + \Gamma)(4 + 5\Gamma)\psi^2 - 3(2756 + \Gamma(81544 + 44835\Gamma))\psi^4)}{540672(2 + \Gamma)(2 + 3\Gamma)}, \quad (92)$$

$$H_{11} = \frac{25(4224(4 + \Gamma)(4 + 5\Gamma)\psi^2 - (1252 + \Gamma(70088 + 38955\Gamma))\psi^4)}{360448(2 + \Gamma)(2 + 3\Gamma)}, \quad (93)$$

$$H_{12} = \frac{175(528(4 + \Gamma)(4 + 5\Gamma)\psi^2 + (652 - \Gamma(7144 + 4263\Gamma))\psi^4)}{180224(2 + \Gamma)(2 + 3\Gamma)}, \quad (94)$$

$$H_{13} = -\frac{539}{64}H_9, H_{14} = \frac{125\psi^2(-792(4 + \Gamma)(4 + 5\Gamma) + (6052 + \Gamma(24776 + 11667\Gamma))\psi^2)}{67584(2 + \Gamma)(2 + 3\Gamma)}, \quad (95)$$

$$H_{15} = \frac{525\psi^2(-22(4 + \Gamma)(4 + 5\Gamma) + (228 + \Gamma(808 + 369\Gamma))\psi^2)}{5632(2 + \Gamma)(2 + 3\Gamma)}, \quad (96)$$

$$H_{16} = \frac{539}{12}H_9, H_{17} = -\frac{151}{4}H_9, H_{18} = -\frac{539}{12}H_9, H_{19} = -\frac{3(1 + \psi^2)}{2(2 + 3\Gamma)}, \quad (97)$$

$$H_{20} = \frac{12 + 5\psi^2}{16 + 24\Gamma}, H_{21} = \frac{35\psi^2}{16 + 24\Gamma}, H_{22} = -\frac{35\psi^2}{8 + 12\Gamma}, \quad (98)$$

$$I_1 = -\frac{2}{5}H_9, I_2 = \frac{1}{11264(2+\Gamma)(2+3\Gamma)} [3(-4224(5+2\Gamma(4+\Gamma)) - 44(480+\Gamma(472+53\Gamma)))\psi^2 + (1340+3\Gamma(3944+2051\Gamma))\psi^4], \quad (99)$$

$$I_3 = \frac{5\psi^2(99\Gamma(8+7\Gamma) + 4(199+794\Gamma+372\Gamma^2)\psi^2)}{8448(2+\Gamma)(2+3\Gamma)}, \quad (100)$$

$$I_4 = \frac{35(-132(4+\Gamma)(4+5\Gamma)\psi^2 + (-604+\Gamma(904+735\Gamma))\psi^4)}{22528(2+\Gamma)(2+3\Gamma)}, \quad (101)$$

$$I_5 = \frac{35\psi^2(-33(4+\Gamma)(4+5\Gamma) + 2(-74+\Gamma(116+93\Gamma))\psi^2)}{5632(2+\Gamma)(2+3\Gamma)}, I_6 = \frac{211}{15}H_9, \quad (102)$$

$$I_7 = \frac{77}{3}H_9, I_8 = \frac{5(3168(4+\Gamma)(4+5\Gamma)\psi^2 - 9(4596+\Gamma(14824+6615\Gamma))\psi^4)}{135168(2+\Gamma)(2+3\Gamma)}, \quad (103)$$

$$I_9 = \frac{35(264(4+\Gamma)(4+5\Gamma)\psi^2 + (788-\Gamma(2648+1785\Gamma))\psi^4)}{11264(2+\Gamma)(2+3\Gamma)}, I_{10} = -\frac{77}{8}H_9, \quad (104)$$

$$I_{11} = -\frac{5\psi^2(264(4+\Gamma)(4+5\Gamma) + (6196+\Gamma(8168+2271\Gamma))\psi^2)}{11264(2+\Gamma)(2+3\Gamma)}, \quad (105)$$

$$I_{12} = \frac{35\psi^2(66(4+\Gamma)(4+5\Gamma) + (284-\Gamma(488+381\Gamma))\psi^2)}{2816(2+\Gamma)(2+3\Gamma)}, I_{13} = -\frac{77}{6}H_9, \quad (106)$$

$$I_{14} = \frac{3(1+\psi^2)}{4(2+3\Gamma)}, I_{15} = \frac{24+45\psi^2}{64+96\Gamma}, I_{16} = \frac{35\psi^2}{64+96\Gamma}, I_{17} = \frac{65\psi^2}{64+96\Gamma}, I_{18} = \frac{7}{13}I_{17}, \quad (107)$$

$$J_1 = \frac{5\psi^2(198(40+\Gamma(56+9\Gamma)) + (1340-\Gamma(6824+4341\Gamma))\psi^2)}{8448(2+\Gamma)(2+3\Gamma)}, \quad (108)$$

$$J_2 = \frac{5\psi^2(198(72+\Gamma(104+19\Gamma)) + (3284-\Gamma(9272+6447\Gamma))\psi^2)}{8448(2+\Gamma)(2+3\Gamma)}, \quad (109)$$

$$J_3 = \frac{2}{5}H_9, J_4 = \frac{25\psi^2(-396(4+\Gamma)(4+5\Gamma) + (716+\Gamma(7768+4101\Gamma))\psi^2)}{16896(2+\Gamma)(2+3\Gamma)}, \quad (110)$$

$$J_5 = \frac{35\psi^2(-99(4+\Gamma)(4+5\Gamma) + (344+\Gamma(2272+1149\Gamma))\psi^2)}{4224(2+\Gamma)(2+3\Gamma)}, J_6 = 11H_9, \quad (111)$$

$$J_7 = -\frac{266}{15}H_9, J_8 = -22H_9, J_9 = -\frac{25\psi^2}{8+12\Gamma}, \quad (112)$$

$$K_1 = -\frac{(1+3\cos 2\theta)}{64(2+\Gamma)(2+3\Gamma)} [-72(5+2\Gamma(4+\Gamma)) - 3(100+\Gamma(88+7\Gamma))\psi^2 + 4(10+\Gamma(44+21\Gamma))\psi^4] + \frac{5}{96} [\psi^2(9+8\psi^2)\cos 2\phi \sin^2 \theta], \quad (113)$$

$$K_2 = \frac{63(-132(4+\Gamma)(4+5\Gamma)\psi^2 + (-604+\Gamma(904+735\Gamma))\psi^4)}{22528(2+\Gamma)(2+3\Gamma)}, \quad (114)$$

$$K_3 = \frac{20}{9}K_2, K_4 = \frac{35}{9}K_2, \quad (115)$$

$$K_5 = \frac{175\psi^2(33(4+\Gamma)(4+5\Gamma) - 2(-74+\Gamma(116+93\Gamma))\psi^2)}{1408(2+\Gamma)(2+3\Gamma)}, \quad (116)$$

$$K_6 = \frac{7}{5}K_5, K_7 = \frac{14}{5}H_9, \quad (117)$$

$$K_8 = \frac{174\psi^4}{49152} [-3(50 + 105 \cos 2\theta + 126 \cos 4\theta + 231 \cos 6\theta) + 112(35 + 60 \cos 2\theta + 33 \cos 4\theta) \cos 2\phi \sin^2 \theta - 336(9 + 11 \cos 2\theta) \cos 4\phi \sin^4 \theta] \quad (118)$$

$$K_9 = -\frac{3(1 + \psi^2)}{2(2 + 3\Gamma)}, K_{10} = -\frac{35\psi^2}{32 + 48\Gamma}, K_{11} = 10K_{10}, \quad (119)$$

$$L_1 = -\frac{1}{2162688(2 + \Gamma)^2(2 + 3\Gamma)^2(14 + 17\Gamma)(14 + 19\Gamma)} [304128(14 + 17\Gamma)(7840 + \Gamma(33504 + \Gamma(53806 + \Gamma(40067 + \Gamma(13704 + 1739\Gamma))))) + 6336(5509504 + \Gamma(27914608 + \Gamma(56856960 + \Gamma(59270984 + \Gamma(33048488 + 9208023\Gamma + 992088\Gamma^2)))))\psi^2 + 3(3828969536 + \Gamma(19657251968 + \Gamma(40731330192 + \Gamma(43445669056 + \Gamma(25023158572 + 9\Gamma(813558984 + 94192115\Gamma)))))\psi^4], \quad (120)$$

$$L_2 = \frac{1}{1441792(2 + \Gamma)^2(2 + 3\Gamma)^2(14 + 17\Gamma)(14 + 19\Gamma)} [202752(14 + 17\Gamma)(5600 + \Gamma(27360 + \Gamma(50066 + \Gamma(42109 + \Gamma(15864 + 2101\Gamma))))) + 5632(2481920 + \Gamma(15231920 + \Gamma(36584256 + \Gamma(43640392 + \Gamma(26832856 + 7843683\Gamma + 812898\Gamma^2)))))\psi^2 - (2634134720 + \Gamma(10174509440 + \Gamma(21446075568 + \Gamma(34750482496 + \Gamma(35446691908 + 3\Gamma(5917712968 + 1100401563\Gamma)))))\psi^4], \quad (121)$$

$$L_3 = -\frac{5}{720896(2 + \Gamma)(2 + 3\Gamma)(14 + 17\Gamma)} [4928(-208 + \Gamma(-306 + \Gamma(109 + 240\Gamma)))\psi^2 + (-477848 + \Gamma(3199164 + \Gamma(6842534 + 2783505\Gamma)))\psi^4], \quad (122)$$

$$L_4 = \frac{385}{256}H_9, L_5 = \frac{1}{270336(2 + \Gamma)(2 + 3\Gamma)(14 + 17\Gamma)(14 + 19\Gamma)} [5\psi^2(1056(61600 + \Gamma(246476 + \Gamma(360128 + \Gamma(219889 + 43092\Gamma)))) + (145457200 + \Gamma(459208832 + \Gamma(473450696 + \Gamma(169213408 + 13223499\Gamma))))\psi^2], \quad (123)$$

$$L_6 = \frac{1}{22528(2 + \Gamma)(2 + 3\Gamma)(14 + 17\Gamma)} [35\psi^2(-88(-208 + \Gamma(-306 + \Gamma(109 + 240\Gamma))) + 3(10888 + \Gamma(6812 - 3\Gamma(5054 + 3081\Gamma)))\psi^2)], \quad (124)$$

$$L_7 = \frac{385}{48}H_9, L_8 = -\frac{2819}{1680}H_9, L_9 = \frac{385}{48}H_9, L_{10} = \frac{1}{(2 + 3\Gamma)^2}, L_{11} = -\frac{105\psi^2}{128(2 + 3\Gamma)}, \quad (125)$$

$$L_{12} = -\frac{960 + 384\Gamma(4 + \Gamma) + 9(22 + 3\Gamma)(10 + 7\Gamma)\psi^2}{128(2 + \Gamma)(2 + 3\Gamma)^2}, L_{13} = \frac{105\psi^2}{64 + 96\Gamma}. \quad (126)$$

#### 4 Particle translating in the quadratic component of Hagen-Poiseuille flow

The expressions of  $\tilde{A}_n$ ,  $\tilde{E}_n$ ,  $\tilde{F}_n$ ,  $\tilde{H}_n$ ,  $\tilde{I}_n$ ,  $\tilde{K}_n$ , and  $\tilde{L}_n$  in velocity, pressure, displacement, deformation and point force at different orders in  $\alpha$  are obtained as

$$\tilde{A}_1 = \frac{3 + 2\psi^2}{2}, \tilde{A}_2 = -\frac{2 + \psi^2}{4}, \tilde{A}_3 = -\frac{7\psi^2}{4}, \tilde{A}_4 = 0, \tilde{B}_1 = -\frac{1}{4} - \frac{11\psi^2}{32}, \quad (127)$$

$$\tilde{E}_1 = -\frac{3(32(-1 + \Gamma^2) + 2(-2 + 3\Gamma)(22 + 13\Gamma)\psi^2)}{64(2 + \Gamma)(2 + 3\Gamma)}, \quad (128)$$

$$\tilde{F}_1 = -\frac{(3+\Gamma)(3+2\psi^2)}{4(2+\Gamma)}, \tilde{F}_2 = \frac{96(1+\Gamma)(3+2\Gamma) + (932 + \Gamma(1160 + 363\Gamma))\psi^2}{64(2+\Gamma)(2+3\Gamma)}, \quad (129)$$

$$\tilde{H}_1 = \frac{108(5+2\Gamma(4+\Gamma)) + 9(100 + \Gamma(88 + 7\Gamma))\psi^2 - 4(-40 + \Gamma(64 + 51\Gamma))\psi^4}{192(2+\Gamma)(2+3\Gamma)}, \quad (130)$$

$$\tilde{H}_2 = 3\tilde{H}_1, \tilde{H}_3 = 0, \tilde{H}_4 = \frac{1}{16896(2+\Gamma)(2+3\Gamma)} [-9504(5+2\Gamma(4+\Gamma)) - 99(1520 + \Gamma(1784 + 281\Gamma))\psi^2 + (-96700 + \Gamma(-152 + 36177\Gamma))\psi^4], \quad (131)$$

$$\tilde{H}_5 = \frac{1}{1408(2+\Gamma)(2+3\Gamma)} [-2376(5+2\Gamma(4+\Gamma)) - 33(1000 + \Gamma(1128 + 167\Gamma))\psi^2 + (-18820 + \Gamma(1432 + 7863\Gamma))\psi^4], \quad (132)$$

$$\tilde{H}_6 = \frac{525\psi^2(-11(4+\Gamma)(4+5\Gamma) + (-204 + \Gamma(-56 + 45\Gamma))\psi^2)}{5632(2+\Gamma)(2+3\Gamma)}, \quad (133)$$

$$\tilde{H}_7 = \tilde{H}_8 = \tilde{H}_9 = 0, \quad (134)$$

$$\tilde{H}_{10} = \frac{17820(4+\Gamma)(4+5\Gamma)\psi^2 - 5(-41596 + \Gamma(30856 + 32955\Gamma))\psi^4}{67584(2+\Gamma)(2+3\Gamma)}, \quad (135)$$

$$\tilde{H}_{11} = \frac{26400(4+\Gamma)(4+5\Gamma)\psi^2 - 25(-12724 + \Gamma(8344 + 9465\Gamma))\psi^4}{45056(2+\Gamma)(2+3\Gamma)}, \quad (136)$$

$$\tilde{H}_{12} = \frac{525\psi^2(44(4+\Gamma)(4+5\Gamma) + (620 - 3\Gamma(56 + 109\Gamma))\psi^2)}{22528(2+\Gamma)(2+3\Gamma)}, \tilde{H}_{13} = -\frac{8575\psi^4}{4096}, \quad (137)$$

$$\tilde{H}_{14} = \tilde{H}_{15} = \tilde{H}_{16} = \tilde{H}_{17} = \tilde{H}_{18} = 0, \tilde{H}_{19} = -\frac{3+6\psi^2}{4+6\Gamma}, \tilde{H}_{20} = \frac{6+5\psi^2}{8+12\Gamma}, \quad (138)$$

$$\tilde{H}_{21} = \frac{35\psi^2}{8+12\Gamma}, \tilde{H}_{22} = 0, \quad (139)$$

$$\tilde{I}_1 = 0, \tilde{I}_2 = \frac{1}{4224(2+\Gamma)(2+3\Gamma)} [-4752(5+2\Gamma(4+\Gamma)) - 99(480 + \Gamma(472 + 53\Gamma))\psi^2 + (-16220 + \Gamma(8744 + 11001\Gamma))\psi^4], \tilde{I}_3 = 0, \quad (140)$$

$$\tilde{I}_4 = \frac{105\psi^2(-11(4+\Gamma)(4+5\Gamma) + (-204 + \Gamma(-56 + 45\Gamma))\psi^2)}{2816(2+\Gamma)(2+3\Gamma)}, \tilde{I}_5 = 0, \tilde{I}_6 = 0, \quad (141)$$

$$\tilde{I}_7 = 0, \tilde{I}_8 = \frac{3960(4+\Gamma)(4+5\Gamma)\psi^2 - 5(3932 + \Gamma(33208 + 17205\Gamma))\psi^4}{16896(2+\Gamma)(2+3\Gamma)}, \quad (142)$$

$$\tilde{I}_9 = \frac{35\psi^2(66(4+\Gamma)(4+5\Gamma) + (1084 + (56 - 375\Gamma)\Gamma)\psi^2)}{1408(2+\Gamma)(2+3\Gamma)}, \tilde{I}_{10} = -\frac{1225\psi^4}{512}, \quad (143)$$

$$\tilde{I}_{11} = \tilde{I}_{12} = \tilde{I}_{13} = 0, \tilde{I}_{14} = \frac{3+6\psi^2}{8+12\Gamma}, \tilde{I}_{15} = \frac{12+45\psi^2}{32+48\Gamma}, \tilde{I}_{16} = \frac{35\psi^2}{32+48\Gamma}, \quad (144)$$

$$\tilde{I}_{17} = \tilde{I}_{18} = 0, \quad (145)$$

$$\tilde{J}_1 = \tilde{J}_2 = \tilde{J}_3 = \tilde{J}_4 = \tilde{J}_5 = \tilde{J}_6 = \tilde{J}_7 = \tilde{J}_8 = \tilde{J}_9 = 0, \quad (146)$$

$$\tilde{K}_1 = -\frac{(1+3\cos 2\theta)}{96(2+\Gamma)(2+3\Gamma)} [-108(5+2\Gamma(4+\Gamma)) - 9(100+\Gamma(88+7\Gamma))\psi^2 + 4(-40 + \Gamma(64+51\Gamma))\psi^4], \quad (147)$$

$$\tilde{K}_2 = \frac{189\psi^2(-11(4+\Gamma)(4+5\Gamma) + (-204+\Gamma(-56+45\Gamma))\psi^2)}{2816(2+\Gamma)(2+3\Gamma)}, \tilde{K}_3 = \frac{20}{9}\tilde{K}_2, \tilde{K}_4 = \frac{35}{9}\tilde{K}_2, \quad (148)$$

$$\tilde{K}_5 = \tilde{K}_6 = \tilde{K}_7 = 0, \tilde{K}_8 = -\frac{175\psi^4}{6144} [50 + 105\cos 2\theta + 126\cos 4\theta + 231\cos 6\theta], \quad (149)$$

$$\tilde{K}_9 = -\frac{3+6\psi^2}{4+6\Gamma}, \tilde{K}_{10} = -\frac{35\psi^2}{16+24\Gamma}, \tilde{K}_{11} = 0, \quad (150)$$

$$\begin{aligned} \tilde{L}_1 = & -\frac{1}{270336(2+\Gamma)^2(2+3\Gamma)^2(14+17\Gamma)(14+19\Gamma)} [38016(14+17\Gamma)(7840+\Gamma(33504 \\ & +\Gamma(53806+\Gamma(40067+\Gamma(13704+1739\Gamma)))) + 1584(5509504+\Gamma(27914608 \\ & +\Gamma(56856960+\Gamma(59270984+\Gamma(33048488+9208023\Gamma+992088\Gamma^2))))))\psi^2 \\ & + (5070115904+\Gamma(24616380032+\Gamma(47238123408+\Gamma(45319190464+\Gamma(22505491948 \\ & +5306816424\Gamma+434154555\Gamma^2))))))\psi^4], \end{aligned} \quad (151)$$

$$\begin{aligned} \tilde{L}_2 = & \frac{1}{180224(2+\Gamma)^2(2+3\Gamma)^2(14+17\Gamma)(14+19\Gamma)} [25344(14+17\Gamma)(5600+\Gamma(27360 \\ & +\Gamma(50066+\Gamma(42109+\Gamma(15864+2101\Gamma)))) + 1408(2481920+\Gamma(15231920 \\ & +\Gamma(36584256+\Gamma(43640392+\Gamma(26832856+7843683\Gamma+812898\Gamma^2))))))\psi^2 \\ & + (-1107229760+\Gamma(-1815969920+\Gamma(2802466416+\Gamma(7204549952+\Gamma(4230619796 \\ & +3(140791016-54514569\Gamma)\Gamma))))))\psi^4], \end{aligned} \quad (152)$$

$$\begin{aligned} \tilde{L}_3 = & -\frac{1}{90112(2+\Gamma)(2+3\Gamma)(14+17\Gamma)} [6160(-208+\Gamma(-306+\Gamma(109+240\Gamma)))\psi^2 \\ & + 35(-116152+\Gamma(-35124+\Gamma(228046+124125\Gamma)))\psi^4], \end{aligned} \quad (153)$$

$$\tilde{L}_4 = \frac{6125\psi^4}{16384}, \tilde{L}_5 = \tilde{L}_6 = \tilde{L}_7 = \tilde{L}_8 = \tilde{L}_9 = 0, \tilde{L}_{10} = \frac{1}{(2+3\Gamma)^2}, \tilde{L}_{11} = -\frac{105\psi^2}{64(2+3\Gamma)}, \quad (154)$$

$$\tilde{L}_{12} = -\frac{96(5+2\Gamma(4+\Gamma)) + 9(22+3\Gamma)(10+7\Gamma)\psi^2}{64(2+\Gamma)(2+3\Gamma)^2}, \tilde{L}_{13} = 0. \quad (155)$$
